# Supplementary material for: Webots.HPC: A Parallel Robotics Simulation Pipeline for Autonomous Vehicles on High Performance Computing
Source: arXiv:2108.00485 source file (2021-08-01)
Supplement: Supplementary file 2 [file appendixB.tex]

\section{PBS Job Script}
\lstinputlisting[language=bash]{sim_parallel_FORDISPLAY.pbs}
